# Supplementary material for: The Meta Distribution of the SIR in Joint Communication and Sensing Networks
Source: arXiv:2404.01672 source file (2024-04-02)
Supplement: Supplementary file 1 [file 07_AppendixB.tex]

%========================================%
%            Appendix B
%========================================%

\section*{Appendix B: Proof of Corollary \ref{cor:LOSonly_sen_momts}} \label{apx:aprx_momts}

Conditioned on the distance from the typical SO and serving BS, when the NLOS BSs is ignored, the intensity measure of $\Pi^0_\mathrm{b}$ may be simplified into 
\begin{align}
		\lambda_\mathrm{b}^0(r;r_0) = 2 \lambda_\mathrm{b} r(\pi-\arccos(\frac{r}{2r_0})\mathbbm{1}\{r \leq 2r_0\}).
\end{align} 
Then the conditional moment of the sensing  coverage probability can be simplified into 
	\begin{align}\label{equ:Msbr02}
		%M^s_{b|r_0}  \nonumber \\ 
		& M^s_{b|r_0}  =  \exp \Big( -\int_{\mathbb{R}^2}\Big[1-\frac{1}{(1+\theta_{\mathrm{s}} r_0^{2\alpha}r^{-\alpha})^b}\Big]\lambda_\mathrm{b}^0(r;r_0)dr\Big)\nonumber\\
		& \stackrel{(a)}= \exp\Bigg(
		-4\lambda_\mathrm{b} \pi r_0^2\delta\int_{0}^{1}\big(1-\frac{1}{(1+\theta_{\mathrm{s}}(\frac{r_0}{2})^{\frac{2}{\delta}}v)^b}\big)v^{-\delta-1}dv\nonumber\\
		&\quad\quad\quad-2\lambda_\mathrm{b} \pi r_0^2\delta\int_{1}^{\infty}\big(1-\frac{1}{(1+\theta_{\mathrm{s}}(\frac{r_0}{2})^{\frac{2}{\delta}}v)^b}\big)v^{-\delta-1}dv\nonumber\\
		&\quad\quad\quad-4\lambda_\mathrm{b} r_0^2\delta \sum_{n=0}^{\infty} \frac{\Gamma(n+\frac{1}{2})}{\Gamma(\frac{1}{2})n!(1+2n)}\nonumber\\
	 &\quad\quad\quad\times\int_{1}^{\infty}\big(1-\frac{1}{(1+\theta_{\mathrm{s}}(\frac{r_0}{2})^{\frac{2}{\delta}}v)^b}\big)v^{-\delta(n+\frac{3}{2})-1}dv
		\Bigg)\nonumber\\
		& \stackrel{(b)}= \exp(-\lambda_\mathrm{b} F^s_b(r_0) )
	\end{align}
	where step (a) follows by the substitution of $v=(\frac{2r_0}{r})^{\alpha}$ and the Taylor expansion of $\arcsin(x)$, step (b) follows by the algebraic operation
 % of the following integration
    %  \begin{align}\label{equ:C1}
    %     C_1(x,y,z)&= z\int_{0}^{1} \Big(1-\frac{1}{(1+y u)^x}\Big)u^{-z-1}du \nonumber\\
    %     &= {_2F_1}(x,-z;1-z;y) - 1\\ 
    %     \label{equ:C2}
    %     C_2(x,y,z)&=z\int_{1}^{\infty} \Big(1-\frac{1}{(1+y u)^x}\Big)u^{-z-1}du \nonumber\\
    %     &= 1-\left(\frac{z }{y^x(x+z)}\right){_2F_1}(x,x+z;x+z+1;-\frac{1}{y})
    % \end{align}
and $F_b^s(r_0)$ is defined as \eqref{equ:Fsb}.
The proof is completed by de-conditioning on $r_0$ with its pdf which follows a Rayleigh distribution as $f_R(r_0) = 2\pi \lambda_b r_0 e^{-\lambda_b\pi r_0^2}$.
